# Supplementary material for: Gestalt: a Stacking Ensemble for SQuAD2.0
Source: arXiv:2004.07067 source file (2020-04-02)
Supplement: Supplementary file 1 [file b_appendix.tex]

\section{Appendix - Manually Crafted Ensembles}
\label{app:b}
We follow Occam's razor and attempt the following simple techniques for combining level-0 models.
\begin{enumerate}
    \item \textbf{Plurality voting using the top-1 answers:} Each model $m$ gives its top answer $a^{(i)}_m$ for question $q^{(i)}$; answers are normalized (using the same normalization method when computing scores~\cite{squadStarter}) then counted; finally, the normalized answer with the most votes wins.
    
    \item \textbf{Weighted voting using probability scores of the top-1 answers:} similar to \#1 except that each model's vote carries a weight equal to the probability score it gave its answer $P(a^{(i)}_m)$. Even though the probability scores are not calibrated across models, they are still useful.
    
    \item \textbf{Weighted voting using probability scores of top-1 answers and their statistics:} similar to \#2 except that each top answer $a^{(i)}_m$ by model $m$ for question $q^{(i)}$ is weighted by $$\frac{P(a^{(i)}_m) - \mu (P(a^{(i)}_m))}{\sigma (P(a^{(i)}_m))}$$ which measures how well $m$ separates $a^{(i)}_m$ from the rest of answers it produced for $q^{(i)}$. We also experiment with  $P(a^{(i)}_m) - \mathrm{median} (P(a^{(i)}_m))$ instead and report it below as \#3\textprime.
    
    \item \textbf{Plurality voting using the top-$N$ answers:} similar to \#1 except that it considers the bag of all top-$N$ answers produced by all models (order doesn't matter).
    
    \item \textbf{Weighted voting using top-$N$ rank as a penalty:} similar to the top-1 variant (\#2) except that it penalizes lower-ranking answers using a linear scale; the top answer's weight is $N$, the second-best answer's weight is $N - 1$, etc. --- the $N$-th answer's weight is 1.
    
    \item \textbf{Weighted voting using Fibonacci-scale of top-$N$ rank as a penalty}: similar to \#5 except that it uses the Fibonacci scale (using the $n$-th Fibonacci number instead of $n$).
    
    \item \textbf{Weighted voting using probability scores of top-$N$ answers:} a top-$N$ variant of \#2.
    
    \item \textbf{Weighted voting using probability scores of top-$N$ answers and their statistics:} top-$N$ variants of \#3 and \#3\textprime, reported respectively below as \#8 and \#8\textprime.
\end{enumerate}

The results of which are detailed below:

\begin{table}[ht]
    \centering
    \setlength{\tabcolsep}{4pt}
    \begin{tabular}{lllllllllll}
    \textbf{} & \#1 & \#2 & \#3 & \#3\textprime & \#4 & \#5 & \#6 & \#7 & \#8 & \#8\textprime \\
    \toprule
    \textbf{Dev EM} & 83.119 & 84.090 & 83.580 & 84.090 & 18.657 & 31.902 & 78.217 & 84.288 & 83.876 & \textbf{84.337} \\
    \textbf{Dev F1} & 85.463 & 86.134 & 85.726 & 86.149 & 32.588 & 42.538 & 80.618 & 86.256 & 85.947 & \textbf{86.294} \\
    \bottomrule
    \end{tabular}
\end{table}
